# Supplementary material for: Fourth- and fifth-order virial expansion of harmonically trapped fermions at unitarity
Source: arXiv:2104.14440 ancillary file (2021-04-29)
Supplement: Supplementary file 1 [file SupMatTrappedVirial.pdf]

# Supplemental Material for
# Fourth- and fifth-order virial expansion of harmonically trapped fermions at unitarity

Y. Hou,[1] K. J. Morrell,[1] A. J. Czejdo,[1] and J. E. Drut[1]

[1]*Department of Physics and Astronomy, University of North Carolina, Chapel Hill, North Carolina 27599, USA*

(Dated: April 28, 2021)

In these supplemental materials, we elaborate on the details of the formalism to calculate virial coefficients starting from the Suzuki-Trotter-factorized transfer matrices. We provide formulas for those transfer matrices in the relevant interacting subspaces for systems up to 5 particles, show how to relate them to the corresponding canonical partition functions, and explain how to connect the latter to the virial coefficients. In addition, we provide explicit analytic formulas in coarse temporal lattices, which can be applied to arbitrary interaction strength, trap frequency, and spatial dimension.

## CONTENTS

I. Transfer matrices 1
   A. Three-particle space 2
   B. Four-particle space 2
   C. Five-particle space 2

II. Canonical partition functions 3

III. Virial coefficients 4

IV. Analytic form of virial coefficients in coarse temporal lattices 4

References 6

## I. TRANSFER MATRICES

In the main text we showed the form of the Suzuki-Trotter-factorized transfer matrix $\mathcal{M}_{11}$ of the $1+1$ subspace, written in the coordinate representation. We show here how to construct that matrix in more detail and present results for its higher-body counterparts. We will only consider here the subspaces where the interaction plays a role, as the noninteracting subspaces (e.g. those with $N+0$ particles) are trivial.

We begin by defining the product coordinate and harmonic oscillator states for two distinguishable particles in $d$ spatial dimensions

$$|\mathbf{x}_1\mathbf{x}_2) = |\mathbf{x}_1\rangle|\mathbf{x}_2\rangle, \tag{1}$$

$$|\mathbf{n}_1\mathbf{n}_2) = |\mathbf{n}_1\rangle|\mathbf{n}_2\rangle. \tag{2}$$

Using these states, we have $\exp\left(-\tau\hat{V}\right)|\mathbf{x}_1\mathbf{x}_2) = [\mathbb{1} + C\delta(\mathbf{x}_1-\mathbf{x}_2)]|\mathbf{x}_1\mathbf{x}_2)$, where $C = (\exp\left(\tau g/\ell^d\right)-1)\ell^d$, and so we obtain

$$[\mathcal{M}_{11}]_{\mathbf{x}_1,\mathbf{x}_2;\mathbf{y}_1,\mathbf{y}_2} = \sum_{\mathbf{n}_1,\mathbf{n}_2} e^{-\tau\epsilon_2(\mathbf{n}_1,\mathbf{n}_2)}(\mathbf{x}_1\mathbf{x}_2|\mathbf{n}_1\mathbf{n}_2)(\mathbf{n}_1\mathbf{n}_2|\mathbf{y}_1\mathbf{y}_2)\left[\mathbb{1} + C\delta(\mathbf{y}_1-\mathbf{y}_2)\right], \tag{3}$$

where

$$\epsilon_2(\mathbf{n}_1,\mathbf{n}_2) = \sum_{i=1}^{2}\epsilon(\mathbf{n}_i) \tag{4}$$

and

$$\epsilon(\mathbf{n}) = \omega\sum_{j=1}^{d}([\mathbf{n}]_j + 1/2). \tag{5}$$

We can do the sum over $\mathbf{n}_1, \mathbf{n}_2$ using the Mehler kernel:

$$\sum_{\mathbf{n}_1,\mathbf{n}_2} e^{-\tau\epsilon_2(\mathbf{n}_1,\mathbf{n}_2)}(\mathbf{x}_1\mathbf{x}_2|\mathbf{n}_1\mathbf{n}_2)(\mathbf{n}_1\mathbf{n}_2|\mathbf{y}_1\mathbf{y}_2) = \rho(\mathbf{x}_1,\mathbf{y}_1)\rho(\mathbf{x}_2,\mathbf{y}_2) \tag{6}$$

where the kernel is, as shown in the main text and repeated here for reference,

$$\rho(\mathbf{x},\mathbf{y}) = \sum_{\mathbf{n}} e^{-\tau\epsilon(\mathbf{n})}\phi_{\mathbf{n}}(\mathbf{x})\phi_{\mathbf{n}}(\mathbf{y}) = \frac{1}{\lambda_T^d}\left[\frac{\beta\omega}{\sinh(\tau\omega)}\right]^{d/2}\exp\left[-\mathbf{Z}^T B\mathbf{Z}\right], \tag{7}$$

where $\lambda_T = \sqrt{2\pi\beta}$, $\mathbf{Z}^T = (\mathbf{x}^T/\lambda_T, \mathbf{y}^T/\lambda_T)$, and

$$B = \frac{\pi\beta\omega}{\sinh(\tau\omega)}\begin{pmatrix} \cosh(\tau\omega)\mathbb{1} & -\mathbb{1} \\ -\mathbb{1} & \cosh(\tau\omega)\mathbb{1} \end{pmatrix}, \tag{8}$$

where $\mathbb{1}$ is a $d\times d$ unit matrix.

### A. Three-particle space

Here we will need

$$\exp\left(-\tau\hat{V}\right)|\mathbf{X}) = \left[\mathbb{1} + C(\delta(\mathbf{x}_1-\mathbf{x}_3)+\delta(\mathbf{x}_2-\mathbf{x}_3))\right]|\mathbf{X}), \tag{9}$$

where $\mathbf{X} = (\mathbf{x}_1,\mathbf{x}_2,\mathbf{x}_3)$ is a collective index, and we use $|\mathbf{X})$ to denote a state of distinguishable particles (i.e. no antisymmetrization among the $\mathbf{x}_i$ labels). We thus obtain

$$[\mathcal{M}_{21}]_{\mathbf{x}_1,\mathbf{x}_2,\mathbf{x}_3;\mathbf{y}_1,\mathbf{y}_2,\mathbf{y}_3} = \rho(\mathbf{x}_1,\mathbf{y}_1)\rho(\mathbf{x}_2,\mathbf{y}_2)\rho(\mathbf{x}_3,\mathbf{y}_3)\left[\mathbb{1} + C(\delta(\mathbf{y}_1-\mathbf{y}_3)+\delta(\mathbf{y}_2-\mathbf{y}_3))\right]. \tag{10}$$

### B. Four-particle space

Here we distinguish the 3+1 subspace from the 2+2 subspace.
For the 3+1 case,

$$\exp\left(-\tau\hat{V}\right)|\mathbf{X}) = \left[\mathbb{1} + C(\delta(\mathbf{x}_1-\mathbf{x}_4)+\delta(\mathbf{x}_2-\mathbf{x}_4)+\delta(\mathbf{x}_3-\mathbf{x}_4))\right]|\mathbf{X}), \tag{11}$$

where $\mathbf{X} = (\mathbf{x}_1,\mathbf{x}_2,\mathbf{x}_3,\mathbf{x}_4)$, and so we obtain

$$[\mathcal{M}_{31}]_{\mathbf{X},\mathbf{Y}} = \rho(\mathbf{x}_1,\mathbf{y}_1)\rho(\mathbf{x}_2,\mathbf{y}_2)\rho(\mathbf{x}_3,\mathbf{y}_3)\rho(\mathbf{x}_4,\mathbf{y}_4)\left[\mathbb{1} + C(\delta(\mathbf{y}_1-\mathbf{y}_4)+\delta(\mathbf{y}_2-\mathbf{y}_4)+\delta(\mathbf{y}_3-\mathbf{y}_4))\right]. \tag{12}$$

For the 2+2 case, on the other hand,

$$\begin{aligned}\exp\left(-\tau\hat{V}\right)|\mathbf{X}) = \big[\mathbb{1} &+ C(\delta(\mathbf{x}_1-\mathbf{x}_3)+\delta(\mathbf{x}_1-\mathbf{x}_4)+\delta(\mathbf{x}_2-\mathbf{x}_3)+\delta(\mathbf{x}_2-\mathbf{x}_4)) \\ &+ C^2(\delta(\mathbf{x}_1-\mathbf{x}_3)\delta(\mathbf{x}_2-\mathbf{x}_4)+\delta(\mathbf{x}_1-\mathbf{x}_4)\delta(\mathbf{x}_2-\mathbf{x}_3))\big]|\mathbf{X}),\end{aligned} \tag{13}$$

such that

$$\begin{aligned}&[\mathcal{M}_{22}]_{\mathbf{X},\mathbf{Y}} = \rho(\mathbf{x}_1,\mathbf{y}_1)\rho(\mathbf{x}_2,\mathbf{y}_2)\rho(\mathbf{x}_3,\mathbf{y}_3)\rho(\mathbf{x}_4,\mathbf{y}_4)\times \\ &\left[\mathbb{1} + C(\delta(\mathbf{y}_1-\mathbf{y}_3)+\delta(\mathbf{y}_1-\mathbf{y}_4)+\delta(\mathbf{y}_2-\mathbf{y}_3)+\delta(\mathbf{y}_2-\mathbf{y}_4)) + C^2(\delta(\mathbf{y}_1-\mathbf{y}_3)\delta(\mathbf{y}_2-\mathbf{y}_4)+\delta(\mathbf{y}_1-\mathbf{y}_4)\delta(\mathbf{y}_2-\mathbf{y}_3))\right]\end{aligned} \tag{14}$$

### C. Five-particle space

Here we distinguish the 4+1 subspace from the 3+2 subspace.
For the 4+1 case,

$$\exp\left(-\tau\hat{V}\right)|\mathbf{X}) = \left[\mathbb{1} + C(\delta(\mathbf{x}_1-\mathbf{x}_5)+\delta(\mathbf{x}_2-\mathbf{x}_5)+\delta(\mathbf{x}_3-\mathbf{x}_5)+\delta(\mathbf{x}_4-\mathbf{x}_5))\right]|\mathbf{X}), \tag{15}$$

where $\mathbf{X} = (\mathbf{x}_1, \mathbf{x}_2, \mathbf{x}_3, \mathbf{x}_4, \mathbf{x}_5)$, such that

$$[\mathcal{M}_{41}]_{\mathbf{X},\mathbf{Y}} = \rho(\mathbf{x}_1,\mathbf{y}_1)\rho(\mathbf{x}_2,\mathbf{y}_2)\rho(\mathbf{x}_3,\mathbf{y}_3)\rho(\mathbf{x}_4,\mathbf{y}_4)\rho(\mathbf{x}_5,\mathbf{y}_5) \times \\ [\mathbb{1} + C(\delta(\mathbf{y}_1-\mathbf{y}_5) + \delta(\mathbf{y}_2-\mathbf{y}_5) + \delta(\mathbf{y}_3-\mathbf{y}_5) + \delta(\mathbf{y}_4-\mathbf{y}_5))] \tag{16}$$

For the 3+2 case, on the other hand,

$$\exp\left(-\tau\hat{V}\right)|\mathbf{X}) = [\mathbb{1} + C(\delta(\mathbf{x}_1-\mathbf{x}_4) + \delta(\mathbf{x}_1-\mathbf{x}_5) + \delta(\mathbf{x}_2-\mathbf{x}_4) + \delta(\mathbf{x}_2-\mathbf{x}_5) + \delta(\mathbf{x}_3-\mathbf{x}_4) + \delta(\mathbf{x}_3-\mathbf{x}_5)) + \\ C^2(\delta(\mathbf{x}_1-\mathbf{x}_4)\delta(\mathbf{x}_2-\mathbf{x}_5) + \delta(\mathbf{x}_1-\mathbf{x}_5)\delta(\mathbf{x}_2-\mathbf{x}_4) + \delta(\mathbf{x}_1-\mathbf{x}_4)\delta(\mathbf{x}_3-\mathbf{x}_5) + \\ \delta(\mathbf{x}_1-\mathbf{x}_5)\delta(\mathbf{x}_3-\mathbf{x}_4)]\,|\mathbf{X}), \tag{17}$$

such that

$$[\mathcal{M}_{32}]_{\mathbf{X},\mathbf{Y}} = \rho(\mathbf{x}_1,\mathbf{y}_1)\rho(\mathbf{x}_2,\mathbf{y}_2)\rho(\mathbf{x}_3,\mathbf{y}_3)\rho(\mathbf{x}_4,\mathbf{y}_4)\rho(\mathbf{x}_5,\mathbf{y}_5) \times \\ [\mathbb{1} + C(\delta(\mathbf{y}_1-\mathbf{y}_4) + \delta(\mathbf{y}_1-\mathbf{y}_5) + \delta(\mathbf{y}_2-\mathbf{y}_4) + \delta(\mathbf{y}_2-\mathbf{y}_5) + \delta(\mathbf{y}_3-\mathbf{y}_4) + \delta(\mathbf{y}_3-\mathbf{y}_5)) + \\ C^2(\delta(\mathbf{y}_1-\mathbf{y}_4)\delta(\mathbf{y}_2-\mathbf{y}_5) + \delta(\mathbf{y}_1-\mathbf{y}_5)\delta(\mathbf{y}_2-\mathbf{y}_4) + \delta(\mathbf{y}_1-\mathbf{y}_4)\delta(\mathbf{y}_3-\mathbf{y}_5) + \delta(\mathbf{y}_1-\mathbf{y}_5)\delta(\mathbf{y}_3-\mathbf{y}_4)] \tag{18}$$

## II. CANONICAL PARTITION FUNCTIONS

As anticipated in the main text, the canonical partition functions $Q_{ab}$ for $a$ particles of spin-$\uparrow$ and $b$ particles of spin-$\downarrow$ are obtained from the above transfer matrices by taking the $N_\tau$-th power of the $\mathcal{M}_{ab}$ that appear above and properly antisymmetrizing at the end as needed. One thus obtains the following identities:

$$Q_{11} = \sum_{ab} \left[\mathcal{M}_2^{N_\tau}\right]_{ab,ab}, \tag{19}$$

$$Q_{21} = \frac{1}{2!}\sum_{abc} \left[\left[\mathcal{M}_3^{N_\tau}\right]_{abc,abc} - \left[\mathcal{M}_3^{N_\tau}\right]_{abc,bac}\right], \tag{20}$$

$$Q_{31} = \frac{1}{3!}\sum_{abcd} \left[\left[\mathcal{M}_4^{N_\tau}\right]_{abcd,abcd} - 3\left[\mathcal{M}_4^{N_\tau}\right]_{abcd,bacd} + 2\left[\mathcal{M}_4^{N_\tau}\right]_{abcd,bcad}\right], \tag{21}$$

$$Q_{22} = \frac{1}{(2!)^2}\sum_{abcd} \left[\left[\mathcal{M}_4^{N_\tau}\right]_{abcd,abcd} - 2\left[\mathcal{M}_4^{N_\tau}\right]_{abcd,abdc} + \left[\mathcal{M}_4^{N_\tau}\right]_{abcd,badc}\right], \tag{22}$$

$$Q_{41} = \frac{1}{4!}\sum_{abcde} \left[\left[\mathcal{M}_5^{N_\tau}\right]_{abcde,abcde} - 6\left[\mathcal{M}_5^{N_\tau}\right]_{abcde,abdce} + 3\left[\mathcal{M}_5^{N_\tau}\right]_{abcde,badce} \right. \\ \left. +8\left[\mathcal{M}_5^{N_\tau}\right]_{abcde,acdbe} - 6\left[\mathcal{M}_5^{N_\tau}\right]_{abcde,bcdae}\right], \tag{23}$$

$$Q_{32} = \frac{1}{3!2!}\sum_{abcde} \left[\left[\mathcal{M}_5^{N_\tau}\right]_{abcde,abcde} - 3\left[\mathcal{M}_5^{N_\tau}\right]_{abcde,acbde} + 2\left[\mathcal{M}_5^{N_\tau}\right]_{abcde,bcade} \right. \\ \left. -\left[\mathcal{M}_5^{N_\tau}\right]_{abcde,abced} + 3\left[\mathcal{M}_5^{N_\tau}\right]_{abcde,acbed} - 2\left[\mathcal{M}_5^{N_\tau}\right]_{abcde,bcaed}\right]. \tag{24}$$

In practice, the above expressions are evaluated symbolically, discarding the leading noninteracting contribution (see below).

## III. VIRIAL COEFFICIENTS

The change in the subspace virial coefficients $\Delta b_{ab}$ is obtained by combining the above formulas into

$$\Delta b_{11} = \frac{\Delta Q_{11}}{Q_1}, \tag{25}$$

$$\Delta b_{21} = \frac{\Delta Q_{21}}{Q_1} - \frac{\Delta Q_{11}}{2}, \tag{26}$$

$$\Delta b_{31} = \frac{\Delta Q_{31}}{Q_1} - \frac{\Delta Q_{21}}{2} - \Delta Q_{11}\left(\frac{Q_{20}}{Q_1} - \frac{Q_1}{4}\right), \tag{27}$$

$$\Delta b_{22} = \frac{\Delta Q_{22}}{Q_1} - \Delta Q_{21} - \frac{\Delta(Q_{11}^2)}{2Q_1} + \frac{\Delta Q_{11} Q_1}{2}, \tag{28}$$

$$\Delta b_{41} = \frac{\Delta Q_{41}}{Q_1} - \frac{\Delta Q_{31}}{2} - \Delta Q_{21}\left(\frac{Q_{20}}{Q_1} - \frac{Q_1}{4}\right) - \Delta Q_{11}\left(\frac{Q_{30}}{Q_1} - Q_{20} + \frac{Q_1^2}{8}\right), \tag{29}$$

$$\Delta b_{32} = \frac{\Delta Q_{32}}{Q_1} - \frac{\Delta Q_{31}}{2} - \frac{\Delta Q_{22}}{2} - \frac{\Delta(Q_{21}Q_{11})}{Q_1} - \Delta Q_{21}\left(\frac{Q_{20}}{Q_1} - \frac{3Q_1}{4}\right) + \frac{\Delta(Q_{11}^2)}{2} + \Delta Q_{11}\left(Q_{20} - \frac{3Q_1^2}{8}\right), \tag{30}$$

where we have omitted partition functions of the form $Q_{N0}$ in previous discussions because they correspond to noninteracting systems and are therefore easily obtained. The full $\Delta b_n$, for $n = 2, 3, 4, 5$ are calculated from the above as

$$\Delta b_2 = \Delta b_{11}, \tag{31}$$

$$\Delta b_3 = 2\Delta b_{21}, \tag{32}$$

$$\Delta b_4 = 2\Delta b_{31} + \Delta b_{22}, \tag{33}$$

$$\Delta b_5 = 2\Delta b_{41} + 2\Delta b_{32}. \tag{34}$$

For reference, we note that the virial coefficients of noninteracting, harmonically trapped spin-1/2 fermions in $d$ spatial dimensions are given by

$$b_n^0 = \frac{(-1)^{n+1}}{n}\left(\frac{\sinh(\beta\omega/2)}{\sinh(\beta\omega n/2)}\right)^d. \tag{35}$$

## IV. ANALYTIC FORM OF VIRIAL COEFFICIENTS IN COARSE TEMPORAL LATTICES

As anticipated in the main text, we provide here formulas for the virial coefficients, broken down by their subspace contributions as above, calculated in coarse temporal lattices namely $N_\tau = 1, 2$, for arbitrary spatial dimension $d$, trapping frequency $\beta\omega$, and coupling strength (parametrized by $\Delta b_2$). For completeness, we cite here the results shown in the main text as well.

For $N_\tau = 1$, we find

$$\Delta b_{11} = \frac{C}{\lambda_T^d}\left(\frac{\beta\omega}{\sinh(\beta\omega)}\right)^{d/2}\frac{1}{2\times 2^{d/2}}, \tag{36}$$

$$\Delta b_{21} = -\frac{\Delta b_2}{[2\cosh(\beta\omega)+1]^{d/2}}, \tag{37}$$

$$\Delta b_{31} = \frac{2^{-d/2}\Delta b_2}{\cosh^{d/2}(\beta\omega)\,[2\cosh(\beta\omega)+1]^{d/2}}, \tag{38}$$

$$\Delta b_{22} = \frac{2^{-3d/2}\Delta b_2}{\cosh^{d/2}(\beta\omega)\cosh^d(\beta\omega/2)}\left\{1 + 2^{d/2}\Delta b_2\left[\cosh^{d/2}(\beta\omega) - 2^{d/2+1}\cosh^d(\beta\omega/2)\right]\right\}, \tag{39}$$

$$\Delta b_{41} = -\frac{2^{-d/2}\Delta b_2}{\cosh^{d/2}(\beta\omega)\,[2\cosh(\beta\omega)+2\cosh(2\beta\omega)+1]^{d/2}}, \tag{40}$$

and

$$\begin{aligned}\Delta b_{32} = &-\Delta b_2\left[\frac{\cosh(\beta\omega)-1}{2\cosh^2(2\beta\omega)-\cosh(\beta\omega)-1}\right]^{d/2}\\ &+2(\Delta b_2)^2\left\{\frac{1}{[1+2\cosh(\beta\omega)+2\cosh(2\beta\omega)]^{d/2}}+\frac{2^d}{[7+8\cosh(2\beta\omega)]^{d/2}}\right.\\ &\left.-\frac{2^d}{[11+16\cosh(\beta\omega)+8\cosh(2\beta\omega)]^{d/2}}\right\}.\end{aligned} \tag{41}$$

For $N_\tau = 2$, we find

$$\Delta b_{11} = \frac{C}{\lambda_T^d}\left(\frac{\beta\omega}{\sinh(\beta\omega)}\right)^{d/2}\frac{1}{2^{d/2}} + \left(\frac{C}{\lambda_T^d}\right)^2\left(\frac{(\beta\omega)^2}{\sinh^2(\beta\omega/2)}\right)^{d/2}\frac{1}{2^{d+1}} \tag{42}$$

$$\begin{aligned}\Delta b_{21} = &\frac{C}{\lambda_T^d}\left(\frac{\beta\omega}{\sinh(\beta\omega)}\right)^{d/2}\frac{-1}{[2+4\cosh(\beta\omega)]^{d/2}}\\ &+\left(\frac{C}{\lambda_T^d}\right)^2\left(\frac{(\beta\omega)^2}{\sinh^2(\beta\omega/2)}\right)^{d/2}\left\{\frac{1}{2^{d+1}}\frac{1}{[1+2\cosh(\beta\omega)]^{d/2}}+\frac{-1}{[7+8\cosh(\beta\omega)]^{d/2}}\right\}\end{aligned} \tag{43}$$

$$\begin{aligned}\Delta b_{31} = &\frac{C}{\lambda_T^d}\left(\frac{\beta\omega}{\sinh(\beta\omega)}\right)^{d/2}\frac{1}{2^d}\frac{1}{[(1+\cosh(\beta\omega)+\cosh(2\beta\omega))]^{d/2}}\\ &+\left(\frac{C}{\lambda_T^d}\right)^2\left(\frac{(\beta\omega)^2}{\sinh^2(\beta\omega/2)}\right)^{d/2}\left\{\frac{1}{[10+14\cosh(\beta\omega)+8\cosh(2\beta\omega)]^{d/2}}+\frac{-1}{4^d}\frac{1}{[2\cosh^2(\beta\omega/2)\cosh(\beta\omega)]^{d/2}}\right.\\ &\left.+\frac{1}{2^{2d+1}}\frac{1}{[\cosh^2(\beta\omega/2)(1+2\cosh(\beta\omega))]^{d/2}}\right\}\end{aligned} \tag{44}$$

$$\begin{aligned}\Delta b_{22} = &\frac{C}{\lambda_T^d}\left(\frac{\beta\omega}{\sinh(\beta\omega)}\right)^{d/2}\frac{1}{4^d}\frac{1}{[\cosh^2(\beta\omega/2)\cosh(\beta\omega)]^{d/2}}\\ &+\left(\frac{C}{\lambda_T^d}\right)^2\left(\frac{(\beta\omega)^2}{\sinh^2(\beta\omega/2)}\right)^{d/2}\left\{\frac{1}{2^{3d+1}}\frac{1}{[\cosh^4(\beta\omega/2)]^{d/2}}+\frac{-1}{[32\cosh^2(\beta\omega/2)\cosh(\beta\omega)]^{d/2}}\right.\\ &\left.+\frac{2}{[\cosh^2(\beta\omega/2)(16+32\cosh(\beta\omega))]^{d/2}}+\frac{-2}{[10+14\cosh(\beta\omega)+8\cosh(2\beta\omega)]^{d/2}}\right\}\\ &+\left(\frac{C}{\lambda_T^d}\right)^3\left(\frac{(\beta\omega)^3}{\sinh^3(\beta\omega/2)}\right)^{d/2}\left\{\frac{-4}{[24\cosh(\beta\omega/2)+16\cosh(3\beta\omega/2)]^{d/2}}\right.\\ &\left.+\frac{2}{[64\cosh^3(\beta\omega/2)]^{d/2}}+\left[\frac{\sinh(\beta\omega/2)}{8\sinh(2\beta\omega)}\right]^{d/2}\right\}\\ &+\left(\frac{C}{\lambda_T^d}\right)^4\left(\frac{(\beta\omega)^4}{\sinh^4(\beta\omega/2)}\right)^{d/2}\left\{\frac{-1}{[16+32\cosh(\beta\omega)]^{d/2}}+\frac{3}{4}\frac{1}{[64\cosh^2(\beta\omega/2)]^{d/2}}\right\}\end{aligned} \tag{45}$$

$$\Delta b_{41} = \frac{C}{\lambda_T^d}\left(\frac{\beta\omega}{\sinh(\beta\omega)}\right)^{d/2} \frac{-1}{[4(1+2\cosh(\beta\omega)+\cosh(2\beta\omega)+\cosh(3\beta\omega))]^{d/2}}$$
$$+\left(\frac{C}{\lambda_T^d}\right)^2\left(\frac{(\beta\omega)^2}{\sinh^2(\beta\omega/2)}\right)^{d/2}\left\{\frac{-1}{[13+20\cosh(\beta\omega)+14\cosh(2\beta\omega)+8\cosh(3\beta\omega)]^{d/2}}\right.$$
$$+\frac{1}{[4(3+6\cosh(\beta\omega)+4\cosh(2\beta\omega)+2\cosh(3\beta\omega)]^{d/2}}$$
$$+\frac{-1}{[23+40\cosh(\beta\omega)+24\cosh(2\beta\omega)+8\cosh(3\beta\omega)]^{d/2}}$$
$$\left.+\frac{1}{2}\frac{1}{[4\cosh^2(\beta\omega/2)(4+8\cosh(\beta\omega)+8\cosh(2\beta\omega)]^{d/2}}\right\} \quad (46)$$

$$\Delta b_{32} = \frac{C}{\lambda_T^d}\left(\frac{\beta\omega}{\sinh(\beta\omega)}\right)^{d/2}\frac{-1}{[6+12\cosh(\beta\omega)+8\cosh(2\beta\omega)+4\cosh(3\beta\omega)]^{d/2}}$$
$$+\left(\frac{C}{\lambda_T^d}\right)^2\left(\frac{(\beta\omega)^2}{\sinh^2(\beta\omega/2)}\right)^{d/2}\left\{\frac{1}{[4\cosh^2(\beta\omega/2)(4+8\cosh(\beta\omega)+8\cosh(2\beta\omega))]^{d/2}}\right.$$
$$+\frac{1}{[\cosh^2(\beta\omega/2)(28+32\cosh(2\beta\omega))]^{d/2}}+\frac{-1}{[\cosh^2(\beta\omega/2)(44+64\cosh(\beta\omega)+32\cosh(2\beta\omega))]^{d/2}}$$
$$+\frac{-2}{[23+40\cosh(\beta\omega)+24\cosh(2\beta\omega)+8\cosh(3\beta\omega)]^{d/2}}+\frac{1}{[\cosh^2(\beta\omega)(28+32\cosh(\beta\omega))]^{d/2}}$$
$$+\frac{2}{[8\cosh^2(\beta\omega/2)(3+3\cosh(\beta\omega)+4\cosh(2\beta\omega))]^{d/2}}+\frac{-1}{[(1+2\cosh(\beta\omega))^2(7+8\cosh(\beta\omega))]^{d/2}}$$
$$\left.+\frac{1}{2}\frac{1}{[4(3+6\cosh(\beta\omega)+4\cosh(2\beta\omega)+2\cosh(3\beta\omega))]^{d/2}}\right\}$$
$$+\left(\frac{C}{\lambda_T^d}\right)^3\left(\frac{(\beta\omega)^3}{\sinh^3(\beta\omega/2)}\right)^{d/2}\left\{\frac{1}{[\cosh(\beta\omega)(8+32\cosh(\beta\omega))]^{d/2}}\left[\frac{\sinh(\beta\omega/2)}{\sinh(\beta\omega)}\right]^{d/2}\right.$$
$$+\frac{-2}{[76\cosh(\beta\omega/2)+16(3\cosh(3\beta\omega/2)+\cosh(5\beta\omega/2))]^{d/2}}+\frac{-2}{[16\cosh(\beta\omega/2)(1+2\cosh(\beta\omega)+2\cosh(2\beta\omega))]^{d/2}}$$
$$+\frac{2}{[4\cosh(\beta\omega/2)(5+12\cosh(\beta\omega)+8\cosh(2\beta\omega))]^{d/2}}+\frac{6}{[8\cosh(\beta\omega/2)\cosh(\beta\omega)(7+8\cosh(\beta\omega))]^{d/2}}$$
$$\left.+\frac{-4}{[4\cosh(\beta\omega/2)(15+22\cosh(\beta\omega)+8\cosh(2\beta\omega))]^{d/2}}+\frac{1}{[32\cosh^3(\beta\omega/2)(1+4\cosh(\beta\omega))]^{d/2}}\right\}$$
$$+\left(\frac{C}{\lambda_T^d}\right)^4\left(\frac{(\beta\omega)^4}{\sinh^4(\beta\omega/2)}\right)^{d/2}\left\{\frac{-3}{[60+88\cosh(\beta\omega)+32\cosh(2\beta\omega)]^{d/2}}\right.$$
$$+\frac{3}{[41+72\cosh(\beta\omega)+32\cosh(2\beta\omega)]^{d/2}}+\frac{1}{[33+40\cosh(\beta\omega)+32\cosh(2\beta\omega)]^{d/2}}$$
$$+\frac{1}{2}\frac{1}{[16(1+2\cosh(\beta\omega)+2\cosh(2\beta\omega))]^{d/2}}+\frac{-1}{[4(1+4\cosh(\beta\omega))^2]^{d/2}}$$
$$+\frac{-2}{[20+48\cosh(\beta\omega)+32\cosh(2\beta\omega)]^{d/2}}+\frac{2}{[32\cosh^2(\beta\omega/2)(1+4\cosh(\beta\omega))]^{d/2}}$$
$$\left.+\frac{-1}{2}\frac{1}{[(7+8\cosh(\beta\omega))^2]^{d/2}}+\frac{1}{2}\frac{1}{[25+48\cosh(\beta\omega)+32\cosh(2\beta\omega)]^{d/2}}\right\} \quad (47)$$
